# Supplementary material for: Probing star clusters as cosmic ray factories
Source: arXiv:2307.03477 source file (2023-07-07)
Supplement: Supplementary file 1 [file appendix_B.tex]

\chapter*{Appendix A}\label{ch:appendix_a}
\addcontentsline{toc}{chapter}{Appendix A}
\markboth{APPENDIX A}{}

I wrote a lot of code. The following scripts have been developed using my computer, working hard. day after day.
\section*{Function to show an example}
The package {\tt listings} is very useful to present code listings.\\
\begin{spacing}{1.0}
{\fontfamily{pcr}\footnotesize
\begin{lstlisting}[language=Python]
import numpy as np
    
def incmatrix(genl1,genl2):
    m = len(genl1)
    n = len(genl2)
    M = None #to become the incidence matrix
    VT = np.zeros((n*m,1), int)  #dummy variable
    
    #compute the bitwise xor matrix
    M1 = bitxormatrix(genl1)
    M2 = np.triu(bitxormatrix(genl2),1) 

    for i in range(m-1):
        for j in range(i+1, m):
            [r,c] = np.where(M2 == M1[i,j])
            for k in range(len(r)):
                VT[(i)*n + r[k]] = 1;
                VT[(i)*n + c[k]] = 1;
                VT[(j)*n + r[k]] = 1;
                VT[(j)*n + c[k]] = 1;
                
                if M is None:
                    M = np.copy(VT)
                else:
                    M = np.concatenate((M, VT), 1)
                
                VT = np.zeros((n*m,1), int)
    
    return M
\end{lstlisting}
}
\end{spacing}

\section*{Another Function to show an example}
\begin{spacing}{1.0}
{\fontfamily{pcr}\footnotesize
\begin{lstlisting}[language=C]
#include <stdio.h>
int main() {
    int dividend, divisor, quotient, remainder;
    printf("Enter dividend: ");
    scanf("%d", &dividend);
    printf("Enter divisor: ");
    scanf("%d", &divisor);

    // Computes quotient
    quotient = dividend / divisor;

    // Computes remainder
    remainder = dividend % divisor;

    printf("Quotient = %d\n", quotient);
    printf("Remainder = %d", remainder);
    return 0;
}
\end{lstlisting}
}
\end{spacing}

\section*{Another Function to show an example}
\begin{spacing}{1.0}
{\fontfamily{pcr}\footnotesize
\begin{lstlisting}[language=C]
#include <stdio.h>
int main() {
    int dividend, divisor, quotient, remainder;
    printf("Enter dividend: ");
    scanf("%d", &dividend);
    printf("Enter divisor: ");
    scanf("%d", &divisor);

    // Computes quotient
    quotient = dividend / divisor;

    // Computes remainder
    remainder = dividend % divisor;

    printf("Quotient = %d\n", quotient);
    printf("Remainder = %d", remainder);
    return 0;
}
\end{lstlisting}
}
\end{spacing}

\section*{Another Function to show an example}
\begin{spacing}{1.0}
{\fontfamily{pcr}\footnotesize
\begin{lstlisting}[language=C]
#include <stdio.h>
int main() {
    int dividend, divisor, quotient, remainder;
    printf("Enter dividend: ");
    scanf("%d", &dividend);
    printf("Enter divisor: ");
    scanf("%d", &divisor);

    // Computes quotient
    quotient = dividend / divisor;

    // Computes remainder
    remainder = dividend % divisor;

    printf("Quotient = %d\n", quotient);
    printf("Remainder = %d", remainder);
    return 0;
}
\end{lstlisting}
}
\end{spacing}

\section*{Another Function to show an example}
\begin{spacing}{1.0}
{\fontfamily{pcr}\footnotesize
\begin{lstlisting}[language=C]
#include <stdio.h>
int main() {
    int dividend, divisor, quotient, remainder;
    printf("Enter dividend: ");
    scanf("%d", &dividend);
    printf("Enter divisor: ");
    scanf("%d", &divisor);

    // Computes quotient
    quotient = dividend / divisor;

    // Computes remainder
    remainder = dividend % divisor;

    printf("Quotient = %d\n", quotient);
    printf("Remainder = %d", remainder);
    return 0;
}
\end{lstlisting}
}
\end{spacing}
